# Supplementary material for: Excited state preparation on a quantum computer through adiabatic light-matter coupling
Source: arXiv:2511.22324 ancillary file (2026-05-28)
Supplement: Supplementary file 1 [file si.pdf]

# Excited state preparation on a quantum computer through adiabatic light-matter coupling: Supplementary Material

Hugh G. A. Burton<sup>1, a)</sup> and Maria-Andreea Filip<sup>2</sup>

<sup>1)</sup>Department of Chemistry, University College London, London, WC1H 0AJ, U.K.

<sup>2)</sup>Yusuf Hamied Department of Chemistry, University of Cambridge, Lensfield Road, Cambridge, CB2 1EW, U.K.

(Dated: 27 November 2025)

## Supplementary Note 1. Pathway definition to avoid forming polaritonic state

For an electronic state with a permanent dipole, i.e.  $\langle \Psi | \hat{\mu} | \Psi \rangle \neq 0$ , a polaritonic state can form in the limit  $\omega \approx 0$  and  $\lambda \neq 0$ . This polariton is a resonance between the diabatic states  $|\Psi\rangle \otimes |0\rangle$  and  $|\Psi\rangle \otimes |1\rangle$ . In such cases, there is a large non-adiabatic coupling near the start of the adiabatic evolution that causes the time evolved state to become a superposition of the two configurations preventing adiabatic preparation of the excited state. This situation can be avoided by choosing particular adiabatic pathways in the  $(\omega, \lambda)$  space, defined through the functional forms of  $\omega(s)$  and  $\lambda(s)$ , as outlined in this section.

In what follows, we define the diabatic states as  $|A\rangle = |\Psi\rangle \otimes |0\rangle$  and  $|B\rangle = |\Psi\rangle \otimes |1\rangle$ . The nonadiabatic coupling between the two states is given by

$$d_{AB} = \frac{|\langle A | \partial_s \hat{H} | B \rangle|}{|E_B - E_A|^2}. \quad (1)$$

For small  $\omega$ , the energy difference behaves as  $E_B - E_A \sim \omega$ . The Hamiltonian derivative  $\partial_s \hat{H}$  is given through the chain rule as

$$\frac{\partial \hat{H}}{\partial s} = \frac{\partial \hat{H}}{\partial \omega} \frac{\partial \omega}{\partial s} + \frac{\partial \hat{H}}{\partial \lambda} \frac{\partial \lambda}{\partial s}, \quad (2)$$

and the substituent derivatives are obtained from the coupling electron-photon Hamiltonian as

$$\frac{\partial \hat{H}}{\partial \omega} = \hat{b}^\dagger \hat{b} + \frac{\lambda \omega^{-1/2} \hat{\mu}}{2\sqrt{2}} (\hat{b}^\dagger + \hat{b}) \quad \text{and} \quad \frac{\partial \hat{H}}{\partial \lambda} = \frac{\omega^{1/2} \hat{\mu}}{\sqrt{2}} (\hat{b}^\dagger + \hat{b}) + \lambda \hat{\mu}^2. \quad (3)$$

Therefore, the nonadiabatic coupling in the limit  $\omega \rightarrow 0$  behaves as

$$\frac{\langle A | \partial_s \hat{H} | B \rangle}{|E_B - E_A|^2} \sim \frac{\langle \Psi | \hat{\mu} | \Psi \rangle}{\sqrt{2}} \left( \frac{\lambda \omega^{-5/2}}{2} \frac{\partial \omega}{\partial s} + \omega^{-3/2} \frac{\partial \lambda}{\partial s} \right), \quad (4)$$

where terms that preserve the photon number (e.g.,  $\hat{b}^\dagger \hat{b}$  and  $\hat{\mu}^2$ ) have no contribution to the coupling  $\langle A | \partial_s \hat{H} | B \rangle$ .

The formation of a polaritonic state can be avoided by satisfying the condition  $\lim_{s \rightarrow 0} d_{AB} = 0$ . This is achieved if  $\langle \Psi | \hat{\mu} | \Psi \rangle = 0$ , which occurs when the relevant component of dipole operator does not transform as the totally symmetric irreducible representation. Otherwise, we require that

$$\lim_{s \rightarrow 0} \left( \frac{\lambda \omega^{-5/2}}{2} \frac{\partial \omega}{\partial s} + \omega^{-3/2} \frac{\partial \lambda}{\partial s} \right) = 0. \quad (5)$$

One option to satisfy this equation would be to enforce that the two components of the limit Eq (5) vanish simultaneously as

$$\lim_{s \rightarrow 0} \left[ \lambda \omega^{-5/2} \frac{\partial \omega}{\partial s} \right] = 0 \quad \text{and} \quad \lim_{s \rightarrow 0} \left[ \omega^{-3/2} \frac{\partial \lambda}{\partial s} \right] = 0. \quad (6)$$

A suitable family of pathways that satisfies the end points is given by the parametrization  $\omega(s) = \omega_{\max} s$  and  $\lambda(s) = \lambda_{\max} \sin(\pi s)^n$ , where we require  $n > 0$ . It can readily be shown that the two limits are given by

$$\lim_{s \rightarrow 0} \left[ \lambda \omega^{-5/2} \frac{\partial \omega}{\partial s} \right] \propto \lim_{s \rightarrow 0} \left[ \frac{\sin(\pi s)^n}{s^{5/2}} \right] \propto \lim_{s \rightarrow 0} \left[ s^{(n - \frac{5}{2})} \right], \quad (7a)$$

<sup>a)</sup>Electronic mail: [h.burton@ucl.ac.uk](mailto:h.burton@ucl.ac.uk)

$$\lim_{s \rightarrow 0} \left[ \omega^{-3/2} \frac{\partial \lambda}{\partial s} \right] \propto \lim_{s \rightarrow 0} \left[ \frac{\sin(\pi s)^{n-1} \cos(\pi s)}{s^{-3/2}} \right] \propto \lim_{s \rightarrow 0} \left[ s^{(n-\frac{5}{2})} \right]. \quad (7b)$$

From this analysis, the condition to avoid a large non-adiabatic coupling at  $s \rightarrow 0$  becomes  $\lim_{s \rightarrow 0} \left[ s^{(n-\frac{5}{2})} \right] = 0$ , which is satisfied for  $n > 5/2$ . More generally, we require that the Taylor series approximation of  $\lambda$  in terms of  $\omega$  begins at third order. A suitable pathway is thus provided by  $n = 3$ , which is the path definition we have used for all EXASP simulations.

### Supplementary Note 2. Hardware implementation for the two-site Hubbard chain

Here we describe the implementation of EXASP for the Hubbard dimer on a quantum device using 3 qubits. We consider the (2e,2o) subspace represented in the basis of configurations  $\{|L\bar{L}\rangle, |L\bar{R}\rangle, |R\bar{L}\rangle, |R\bar{R}\rangle\}$ , where  $L$  ( $R$ ) correspond to the left (right) site and an overbar indicates a low-spin electron. The electronic Hamiltonian in this basis given as

$$\mathbf{H}_e = \begin{pmatrix} U & -t & -t & 0 \\ -t & 0 & 0 & -t \\ -t & 0 & 0 & -t \\ 0 & -t & -t & U \end{pmatrix}. \quad (8)$$

Defining the dipole matrix elements as  $\langle L|\hat{\mu}|L\rangle = -d$ ,  $\langle R|\hat{\mu}|R\rangle = d$  and  $\langle R|\hat{\mu}|L\rangle = \langle L|\hat{\mu}|R\rangle = 0$ , where  $2d$  is the distance between the two sites, the  $\hat{\mu}$  and  $\hat{\mu}^2$  operators in the (2e,2o) basis are given by

$$\boldsymbol{\mu} = \begin{pmatrix} -2d & 0 & 0 & 0 \\ 0 & 0 & 0 & 0 \\ 0 & 0 & 0 & 0 \\ 0 & 0 & 0 & 2d \end{pmatrix} \quad \text{and} \quad \boldsymbol{\mu}^2 = \begin{pmatrix} 4d^2 & 0 & 0 & 0 \\ 0 & 0 & 0 & 0 \\ 0 & 0 & 0 & 0 \\ 0 & 0 & 0 & 4d^2 \end{pmatrix}. \quad (9)$$

As a 4-dimensional Hilbert space, the electronic system can be encoded using two qubits, while the two-level photon mode is encoded as a third qubit. The electronic Hamiltonian  $\hat{H}_e$ , photon Hamiltonian  $\hat{H}_p$ , and interacting Hamiltonian are encoded as

$$\hat{H}_e = \frac{U}{2}(III + ZZI) - t(XII + IXI), \quad (10a)$$

$$\hat{H}_p = \frac{\omega}{2}(III - IIZ), \quad (10b)$$

$$\hat{H}_{\text{int}} = -d\lambda\sqrt{\frac{\omega}{2}}(IZX + ZIX) + d^2\lambda^2(III + ZZI). \quad (10c)$$

The adiabatic time propagation is implemented using a Trotter expansion as

$$\hat{U}_k(s_k) \approx e^{i d \lambda_k \sqrt{\frac{\omega_k}{2}} \delta T (IZX + ZIX)} e^{i \frac{\omega_k}{2} \delta T IIZ} e^{-i(\frac{U}{2} + d^2 \lambda_k^2) \delta T ZZI} e^{i t \delta T (XII + IXI)}, \quad (11)$$

where  $\omega_k = \omega(s_k)$  and  $\lambda_k = \lambda(s_k)$ . Scalar Hamiltonian terms that lead to a global phase shift can be ignored.

The exact ground-state wavefunction can be expressed as a one-layer tUPS expansion. The single and double excitation operators for this system can be written in the three-qubit encoding as

$$\kappa^{(1)} = -i(IYI + YII), \quad \text{and} \quad \kappa^{(2)} = -i(XYI + YXI), \quad (12)$$

and the exact ground state can then be encoded as

$$|\Psi_0\rangle = \exp(\theta_1 \kappa^{(1)}) \exp(\theta_2 \kappa^{(2)}) |\Phi_0\rangle \quad (13)$$

for the initial electronic qubit state  $|\Phi_0\rangle = |00\rangle$ . The optimal coefficients were identified using statevector variational optimization starting from the ionic Slater determinant  $|L\bar{L}\rangle$ . Note that any initial closed-shell determinant would suffice as the  $|\Phi_0\rangle = \exp(\theta_1 \kappa^{(1)})$  operator optimizes the orbitals of the reference  $|\Phi_0\rangle$ .

Statevector and hardware simulations were performed using QISKIT with the noise model for the `ibmq_torino` quantum chip. Experiments on real quantum hardware employed the `ibmq_torino` quantum chip, which is one of the IBM Quantum Heron processors. The circuit was obtained using the transpilation and optimization routines in QISKIT. Since the experiment only requires three qubits, the circuit was duplicated 40 times in parallel to maximize the use of this 133 qubit chip and the number of affordable measurement shots. 250 measurement shots were performed, giving a total of  $10^5$  measurements using the circuit parallelization. The final electronic energy obtained with statevector and noisy hardware simulations are compared to the

results from hardware experiments in Supplementary Figure 3. Both hardware simulations and experiments show rapid decay of the final energy to the fully mixed state due to hardware noise.

### Supplementary Figures and Tables

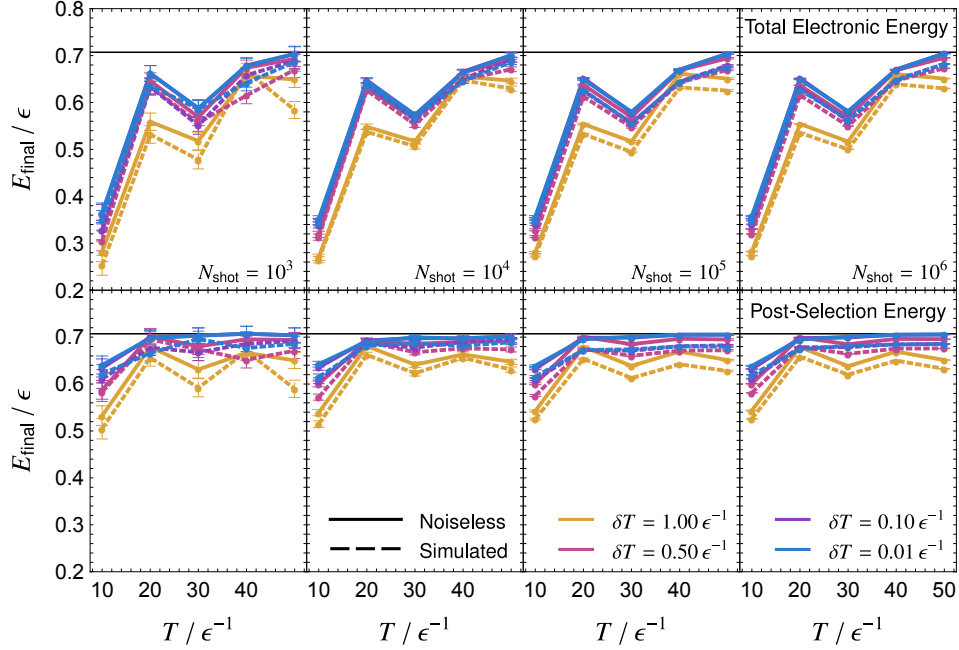

**Supplementary Figure 1: Convergence the final electronic energy for the two-level system.** The system parameters were  $\epsilon = g = \mu = 1$  and the path parameters chosen as  $\omega_{\max} = 5$  and  $\lambda_{\max} = 1$ . Simulated hardware results are based on the noise model for the `ibmq_torin` quantum chip. A time-step satisfying  $\delta T \leq 0.50\epsilon^{-1}$  leads to systematic convergence with respect to the total time evolution  $T$ . These results appear to be convergent with the number of measurement shots for  $N_{\text{shot}} \geq 10^5$ .

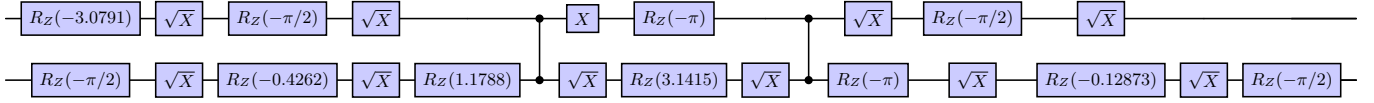

**Supplementary Figure 2: Example optimized circuit for the excited-state preparation in the two-level model.** Regardless of the number of propagation steps, the optimized circuit has a constant depth, meaning that the hardware noise does not increase with the number of propagation steps for this system. Here, the rotation gate parameters correspond to the second iteration

$$s_k = 0.025 \text{ for the two-level model with } \epsilon = g = \mu = 1, T = 20, \delta T = 0.5, \omega_{\max} = 5 \text{ and } \lambda_{\max} = 1.$$

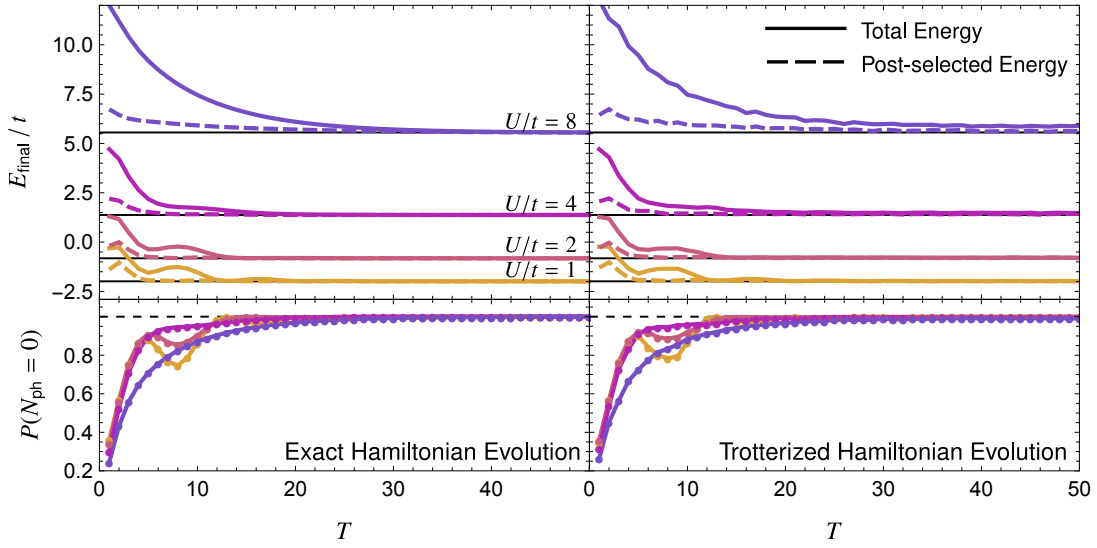

**Supplementary Figure 3: EXASP propagation for the 4-site Hubbard chain.** Convergence of the final total system energy (top) and probability of measuring the  $|0\rangle$  photon state (bottom) at various  $U/t$  values as a function of total evolution time  $T$  with  $\delta T = 0.1$ . Similar convergence is obtained if the propagation is performed exactly or using a first-order Trotter expansion.

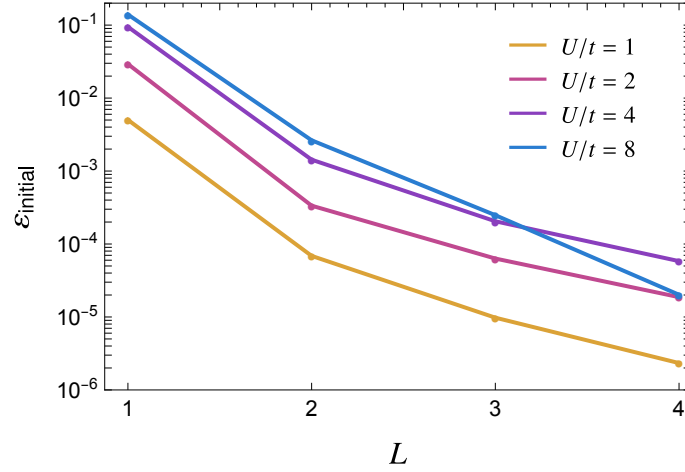

**Supplementary Figure 4: Fidelity error of the pp-tUPS initial state for the 6-site Hubbard chain for  $L$  layers.** The pp-tUPS fidelity error systematically decreases for more layers, but there is an increase in the fidelity error for larger  $U/t$ .

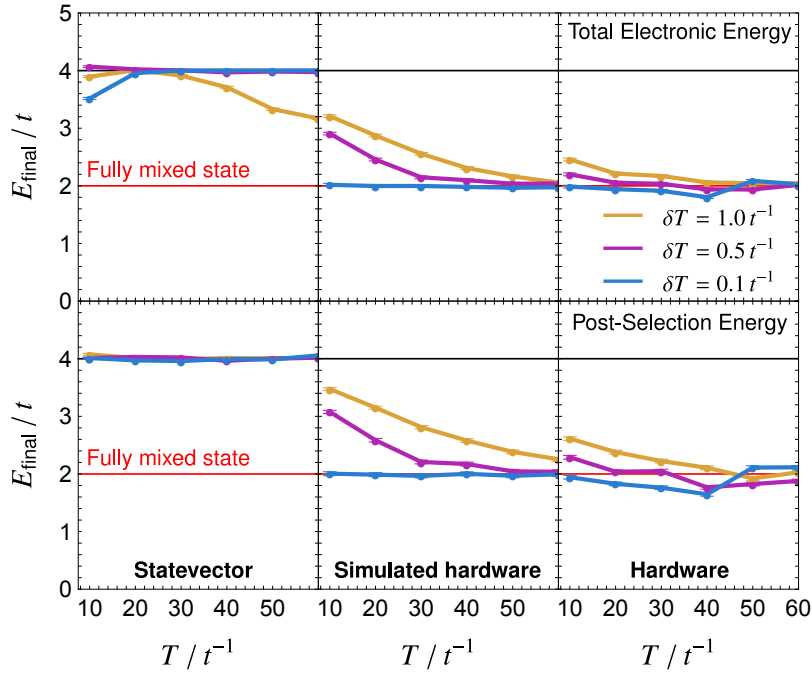

**Supplementary Figure 5: Final electronic energy for the Hubbard dimer computed with a three-qubit hardware experiment.** Simulation parameters are  $U = 4t$  with  $\omega_{\max} = 9.65865$  and  $\lambda_{\max} = 1.0$ . Statevector simulations (left) show that the excited state can be accurately prepared with  $\delta T = 0.5t^{-1}$  and  $T \geq 20t^{-1}$ . However, results from the `ibmq_torino` quantum chip fail to reproduce the final energy and converge rapidly to the fully mixed state (right), demonstrating that there is currently too much hardware noise for accurate excited state preparation.
